# Supplementary material for: Medical Image Analysis using Deep Relational Learning
Source: arXiv:2303.16099 source file (2023-03-28)
Supplement: Supplementary file 1 [file AppendixA.tex]

% Appendix A

\chapter{Ethics Approval Letter}
\label{AppendixA}
 % Main appendix title

University Ethics Sub-Committee for Science and Engineering and Arts Humanities

13/11/2019

Ethics Reference: 19816-lt228-se/in:informatics

TO:
Name of Researcher Applicant: Lei Tong
Department: Computer Science
Research Project Title: Depression Detection Via Twitter

Dear Lei Tong, 

RE: 	Ethics review of Research Study application

The University Ethics Sub-Committee for Science and Engineering and Arts Humanities has reviewed and discussed the above application. 

1.	Ethical opinion

The Sub-Committee grants ethical approval to the above research project on the basis described in the application form and supporting documentation, subject to the conditions specified below.

2.	Summary of ethics review discussion 

The Committee noted the following issues: 
This application has been approved on condition that the further anonymisation procedures outlined in the application are implemented on the dataset.

Best wishes, Martin Phillips

3. 	General conditions of the ethical approval

The ethics approval is subject to the following general conditions being met prior to the start of the project:

As the Principal Investigator, you are expected to deliver the research project in accordance with the University’s policies and procedures, which includes the University’s Research Code of Conduct and the University’s Research Ethics Policy.

If relevant, management permission or approval (gate keeper role) must be obtained from host organisation prior to the start of the study at the site concerned.

4. 	Reporting requirements after ethical approval

You are expected to notify the Sub-Committee about:
•	Significant amendments to the project
•	Serious breaches of the protocol
•	Annual progress reports
•	Notifying the end of the study

5.	Use of application information

Details from your ethics application will be stored on the University Ethics Online System. With your permission, the Sub-Committee may wish to use parts of the application in an anonymised format for training or sharing best practice.  Please let me know if you do not want the application details to be used in this manner.

Best wishes for the success of this research project.

Yours sincerely,

Dr. Martin Phillips 
Chair
