# Supplementary material for: Medical Image Analysis using Deep Relational Learning
Source: arXiv:2303.16099 source file (2023-03-28)
Supplement: Supplementary file 2 [file AppendixB.tex]

\chapter{Appendix of Chapter 4}
\label{AppendixB}
 % Main appendix title
\section{Depression users posting analysis on CLPSych dataset}
\begin{figure*}[htbp]
\centering
\begin{minipage}{\textwidth}
\includegraphics[width=1\textwidth]{Figures/ttdd_tsne_CLP.png}

\label{fig:ttdd_tsne_CLP}
\end{minipage}
\caption{Document representations distribution using TSNE on CLPsych dataset. (a) Top left: Document vectors learned from LDA. (2)Top Right: Document vectors learned from DocNADE. (3) Bottom Left: Document vectors learned from fdp-DocNADE. (4) Bottom Right: Document vectors learned from fdp-DocNADEa.}
\end{figure*}
 
 \begin{figure*}
\centering
\includegraphics[width=0.85\textwidth]{Figures/wordcloud_topics_CLP.png}
\caption{Top probability words in four topics on CLPcych set with manual defined 'theme'}
\label{fig:word_cloud_CLP}
\end{figure*}

Latent Dirichlet Allocation (LDA) is an classical topic model which is shown in  \figurename{\ref{fig:lda_model}. In \figurename{\ref{fig:lda_model}, a dirichlet distribution $\alpha$ represent a particular document and this topic distribution is $\theta$. A particular topic $Z$ can be selected from $\theta$, then the word distribution $\varphi$ of topic $Z$ will be randomly selected from second dirichlet distribution $\beta$.  $N$ is a generated word from $\varphi$ with topic $Z$. The following procedure is to use Gibbs sampling to maximize the loglikehood of $p(W|Z,\varphi)$. In brief, LDA topic model is a clustering process which concentrates on word frequency and word distribution in corpus. Optimized $\theta$ can be represented as document vectors for classification task and word distribution $\varphi$ can be used to describe document content.
\begin{figure*}[htbp]
\centering
\includegraphics[scale=0.5]{Figures/lda_png.png} 
\caption{Latent Dirichlet Allocation (LDA). Image Courtesy of \cite{blei2003latent}} 
\label{fig:lda_model} 
\end{figure*}
