# Supplementary material for: Medical Image Analysis using Deep Relational Learning
Source: arXiv:2303.16099 source file (2023-03-28)
Supplement: Supplementary file 3 [file AppendixTemplate.tex]

% Appendix Template

\chapter{Appendix Title Here} % Main appendix title

\label{AppendixX} % Change X to a consecutive letter; for referencing this appendix elsewhere, use \ref{AppendixX}

Write your Appendix content here.
